# Supplementary material for: Disparity, Inequality, and Accuracy Tradeoffs in Graph Neural Networks for Node Classification
Source: arXiv:2308.09596 source file (2023-08-18)
Supplement: Supplementary file 1 [file appendix_runtime.tex]

\begin{figure}[ht]
	\centering
	\includegraphics[width=0.45\textwidth]{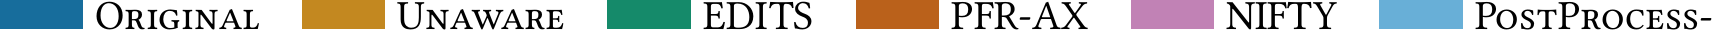}
	\\[2pt]
	\begin{subfigure}{0.45\textwidth}
	  \centering
	  \includegraphics[width=\textwidth]{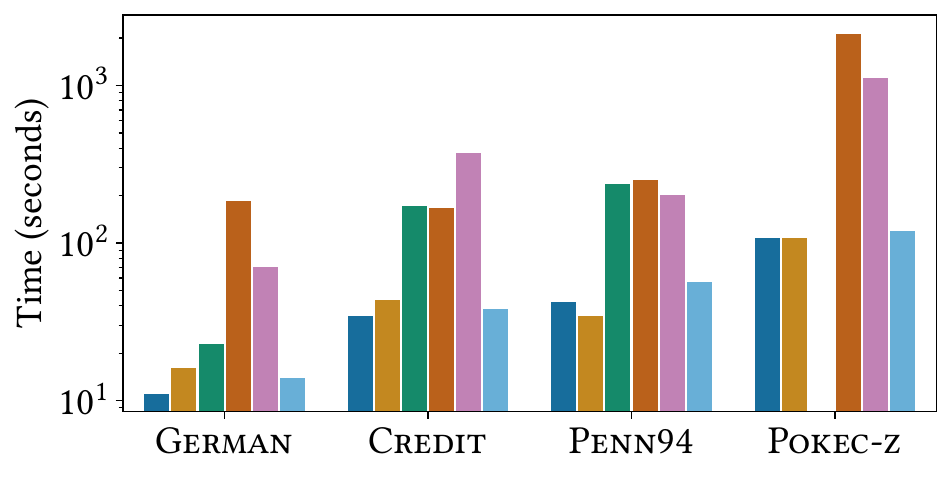}
	  \label{fig:intervention_runtime_GraphSAGE}
	\end{subfigure}
	\caption{Total runtime in seconds (log-scale) of various interventions on \sage for \german, \credit, \penn, and \pokecz datasets.}
	\label{fig:runtime_graphsage}
\end{figure}
